# Supplementary material for: Finite temperature thermodynamic properties of the spin-1 nematics in an applied magnetic field
Source: arXiv:2004.10409 source file (2020-09-16)
Supplement: Supplementary file 1 [file blbq_finiteT_MC_supplemental_v5.pdf]

# Supplemental Material for "Finite temperature thermodynamic properties of the spin-1 nematics in an applied magnetic field"


Katsuhiro Tanaka[1] and Chisa Hotta[1]

[1]*Department of Basic Science, University of Tokyo, Meguro, Tokyo 153-8902, Japan*



(Dated: September 16, 2020)


## I. LOW ENERGY PROPERTIES OF EQ. (4)

Here, the details of how we evaluated the entropy $\tilde{s}(T,h)$ in the main text (Fig. 1(c)) is given.

Our sSU(3)-MC calculation is given for $T \gtrsim 0.2$. In order to evaluate the entropy from the specific heat, one needs to extrapolate these numerical results down to zero temperature. The nematic sSU(3) Hamiltonian Eq. (4) in the main text is formally a classical one that describes the interactions between the complex $\boldsymbol{d}_i$-vectors that represents the local one-body wave function. Similarly to the classical $XY$ models (Refs. [48, 49]), its low-temperature behavior is evaluated by starting from the ground state and considering the low-energy harmonic branches.

The complex $\boldsymbol{d}$-vector on each site can be separated into the real and imaginary parts, $\boldsymbol{d}_i = \boldsymbol{u}_i + \mathrm{i}\boldsymbol{v}_i$, where $\boldsymbol{u}_i, \boldsymbol{v}_i \in \mathbb{R}$. $\boldsymbol{u}_i$ and $\boldsymbol{v}_i$ satisfy the normalization condition, $|\boldsymbol{u}_i|^2 + |\boldsymbol{v}_i|^2 = 1$, and the overall phase can be fixed as $\boldsymbol{u}_i \cdot \boldsymbol{v}_i = 0$ (Refs. [7, 33, 35]). For the ground state with both $h = 0$ and $h \neq 0$, one can choose $\boldsymbol{u}_i$ and $\boldsymbol{v}_i$ to be $\boldsymbol{u}_0$ and $\boldsymbol{v}_0$, whose values do not depend on $i$ and are determined analytically (Refs. [8, 33, 34]). The lowest energy excitations are then obtained by varying these vectors as

$$\boldsymbol{u}_i = \boldsymbol{u}_0 + \delta\boldsymbol{u}_i,\ \boldsymbol{v}_i = \boldsymbol{v}_0 + \delta\boldsymbol{v}_i. \tag{S1}$$

For simplicity, we only consider the case where $(J,K) = (0,-1)$ in the triangular lattice without a magnetic field, while we find shortly that the results do not depend on $h$ or on the bilinear (Heisenberg) terms. The ground state has the ferroquadrupolar order, and $\boldsymbol{u}_0$ and $\boldsymbol{v}_0$ is chosen as

$$\boldsymbol{u}_0 = \begin{pmatrix} 1 \\ 0 \\ 0 \end{pmatrix},\ \boldsymbol{v}_0 = \boldsymbol{0}. \tag{S2}$$

Then, the aforementioned local constraints on $\boldsymbol{u}_i$ and $\boldsymbol{v}_i$ are given as

$$2\delta u_i^x + (\delta\boldsymbol{u}_i)^2 + (\delta\boldsymbol{v}_i)^2 = 0, \qquad \text{(normalization)} \tag{S3}$$

$$\delta v_i^x + \delta\boldsymbol{u}_i \cdot \delta\boldsymbol{v}_i = 0. \qquad \text{(overall phase fixing)} \tag{S4}$$

The energy evaluated by the product state of the one-body wave functions can be rewritten up to $O(\delta^2)$ as

$$\begin{aligned} E_{\mathrm{sSU(3)}} &= -\sum_{\langle i,j\rangle} \left[ (\boldsymbol{u}_i \cdot \boldsymbol{u}_j - \boldsymbol{v}_i \cdot \boldsymbol{v}_j)^2 + (\boldsymbol{u}_i \cdot \boldsymbol{v}_j + \boldsymbol{v}_i \cdot \boldsymbol{u}_j)^2 + 1 \right] \\ &= -zN + \sum_{\langle i,j\rangle} \sum_{\alpha=y,z} \left[ \left( (\delta u_i^\alpha)^2 + (\delta v_i^\alpha)^2 \right) + \left( \left(\delta u_j^\alpha\right)^2 + \left(\delta v_j^\alpha\right)^2 \right) - 2\left( \delta u_i^\alpha \delta u_j^\alpha - \delta v_i^\alpha \delta v_j^\alpha \right) \right], \end{aligned} \tag{S5}$$

Here, we drop the terms including $\delta u_i^x$ and $\delta v_i^x$ using the above constraints. These parameters are Fourier transformed as,

$$\delta\boldsymbol{u}_{\boldsymbol{k}} = \frac{1}{\sqrt{N}} \sum_{i=1}^{N} \mathrm{e}^{-\mathrm{i}\boldsymbol{k}\cdot\boldsymbol{r}_i} \delta\boldsymbol{u}_i,\ \delta\boldsymbol{v}_{\boldsymbol{k}} = \frac{1}{\sqrt{N}} \sum_{i=1}^{N} \mathrm{e}^{-\mathrm{i}\boldsymbol{k}\cdot\boldsymbol{r}_i} \delta\boldsymbol{v}_i, \tag{S6}$$

and the energy $E_{\mathrm{sSU(3)}}$ can be diagonalized as

$$E_{\mathrm{sSU(3)}} = E_0 + \sum_{\boldsymbol{k}} E_{\boldsymbol{k}}, \tag{S7}$$

where

$$E_0 = -zN, \tag{S8}$$

$$E_{\boldsymbol{k}} = \sum_{\alpha=y,z} \left[ (-\gamma_{\boldsymbol{k}} + z)\, \delta u^{\alpha}_{\boldsymbol{k}} \delta u^{\alpha}_{-\boldsymbol{k}} + (\gamma_{\boldsymbol{k}} + z)\, \delta v^{\alpha}_{\boldsymbol{k}} \delta v^{\alpha}_{-\boldsymbol{k}} \right], \tag{S9}$$

$$\gamma_{\boldsymbol{k}} = 2\left[ \cos k_x + \cos\left(\frac{k_x + \sqrt{3}k_y}{2}\right) + \cos\left(\frac{k_x - \sqrt{3}k_y}{2}\right) \right]. \tag{S10}$$

Performing the Gaussian integral, the partition function is calculated as

$$Z \simeq \int \mathrm{e}^{-\beta E_{\mathrm{sSU(3)}}} \prod_{\boldsymbol{k}} \mathrm{d}(\delta u^{y}_{\boldsymbol{k}}) \mathrm{d}(\delta u^{z}_{\boldsymbol{k}}) \mathrm{d}(\delta v^{y}_{\boldsymbol{k}}) \mathrm{d}(\delta v^{z}_{\boldsymbol{k}}) \simeq \mathrm{e}^{-\beta E_0} \prod_{\boldsymbol{k}} \left[ \frac{\pi^2}{\beta^2} \left(\det \mathcal{E}_{\boldsymbol{k}}\right)^{-\frac{1}{2}} \right], \tag{S11}$$

where

$$\det \mathcal{E}_{\boldsymbol{k}} = \begin{pmatrix} -\gamma_{\boldsymbol{k}} + z & & & \\ & -\gamma_{\boldsymbol{k}} + z & & \\ & & \gamma_{\boldsymbol{k}} + z & \\ & & & \gamma_{\boldsymbol{k}} + z \end{pmatrix}. \tag{S12}$$

Then, the statistical average of the energy density, $e(T, h = 0)$, is

$$e(T, h = 0) = \frac{1}{N}\left(-\frac{\partial}{\partial \beta} \ln Z\right) = \frac{E_0}{N} + 2k_{\mathrm{B}}T, \tag{S13}$$

and the specific heat in the low-temperature region, $c(T, h = 0)$, is

$$c(T, h = 0) = \frac{\partial e(T, h = 0)}{\partial T} = 2k_{\mathrm{B}}. \tag{S14}$$

So far, we assumed the particular case $h = 0$ and $J = 0$ with a ferroquadrupolar ground state. However, since this result is nothing but a law of equipartition of energy, the number of low energy modes are responsible, and the same conclusion on $e(T, h)$ and $c(T, h)$ holds even for $h \neq 0$ and $J \neq 0$ as far as the ground state remains ordered, and only the detailed form of $E_0$ and $E_{\boldsymbol{k}}$ is modified. The geometry of the lattice, namely the square lattice, also does not change the result as far as it is in two dimension.

Based on the above consideration, one can assume the temperature dependence of the energy in the low-temeprature region as

$$e(T, h) = e(0, h) + 2k_{\mathrm{B}}T + \alpha(h)T^{\gamma(h)}, \tag{S15}$$

where $e(0, h)$ is the exact ground states energy of $E_{\mathrm{sSU(3)}}$ given in Refs. [8, 33, 34], and $\alpha(h)T^{\gamma(h)}$ with $\gamma(h) > 1$ is the correction beyond $O(\delta^2)$ from Eq. (S13). The actual values of $\alpha(h)$ and $\gamma(h)$ are evaluated by fitting the calculated data. Fitted data is shown in Fig. S1 for $L = 24$ triangular lattice. Then, the specific heat is calculated as

$$c(T, h) = \frac{\partial e(T, h)}{\partial T} = 2k_{\mathrm{B}} + \alpha(h)\gamma(h)T^{\gamma(h)-1}, \tag{S16}$$

and the entropy density is given as

$$s(T, h) = \int_0^T \frac{c(T', h)}{T'} \mathrm{d}T' = \int_0^T \frac{2k_{\mathrm{B}}}{T'} \mathrm{d}T' + \frac{\gamma(h)\alpha(h)}{\gamma(h) - 1} T^{\gamma(h)-1}. \tag{S17}$$

The divergent first term $\int_0^T \frac{2k_{\mathrm{B}}}{T'} \mathrm{d}T'$ is the artifact of dealing with the low energy branches classically. In fact, the original spin-1 BLBQ Hamiltonian (Eq. (1) in the main text) is known to exhibit $T^2$-dependent specific heat at lowest temperature range, which originates from the excitation of three-colored Schwinger bosons (Refs. [8, 33, 40]). This kind of quantum condensation effect is dropped off in $E_{\mathrm{sSU(3)}}$, and instead a classical divergent term appears as an artifact. However, since this term contributes to all cases as common constant shift where the above discussion holds regardless of the values of $h$ and $J$, which no longer plays an important role in discussing the higher temperature range at our focus. We thus drop this term and deal with $\tilde{s}(T, h) = s(T, h) - \int_0^T \frac{2k_{\mathrm{B}}}{T'} \mathrm{d}T'$ in the main text.

We show $e(T, h)$ and $\tilde{s}(T, h)$ obtained by the same treatment for the square lattice in Fig. S2.

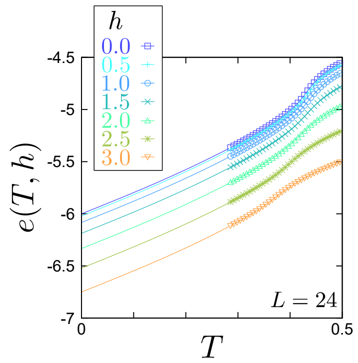


FIG. S1. Energies in the various magnitude of magnetic field in the $L = 24$ triangular lattice with $(J, K) = (0, 1)$. Symbols denote the data obtained by the sSU(3)-MC simulations, and the lines are the energy estimated by fitting the sSU(3)-MC data.

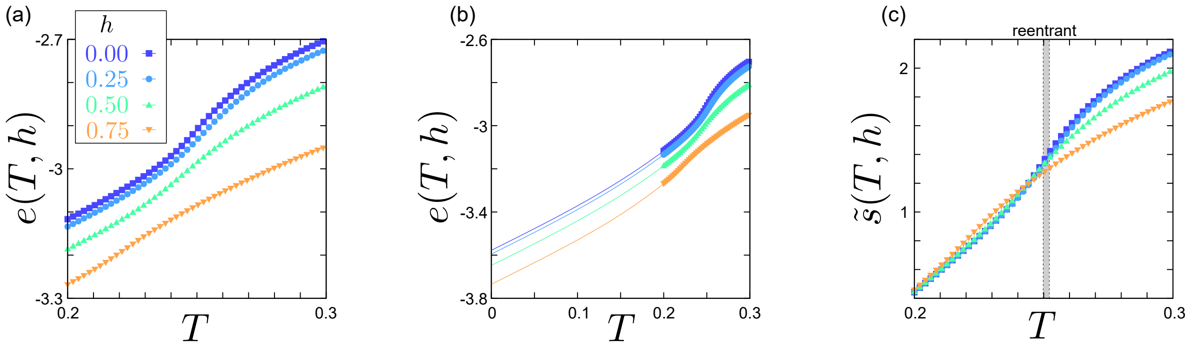


FIG. S2. The evaluated energy and entropy for the $L = 32$ square lattice. The parameters are set as $K/J = 2$ with $J^2 + K^2 = 1$ and $J, K < 0$, i.e., $(J, K) = (-1/\sqrt{5}, -2/\sqrt{5})$. (a) $e(T, h)$ around the phase transition temperature. (b) $e(T, h)$ in the wider temperature region. Lines in the low-temperature region is the energy estimated from the sSU(3)-MC results. (c) Entropy $\tilde{s}(T, h)$ estimated by the above procedure.

## II. DETAILS ON THE FINITE-TEMPERATURE PROPERTIES OF THE FERROQUADRUPOLAR PHASE IN THE SQUARE LATTICE

We show the detailed results of the semiclassical SU(3) Monte Carlo (sSU(3)-MC) simulation (Ref. [31]) for the ferroquadrupolar phase in the square lattice with $L = 32$ (Fig. S3). The parameters are set as $K/J = 2$ with $J, K < 0$, i.e., $(J, K) = (-1/\sqrt{5}, -2/\sqrt{5})$, where the variational ground state is the ferroquadrupolar phase in the absence of the magnetic field (Refs. [33, 34]). $T$–$h$ phase diagram and the temperature dependence of the specific heat are given in Figs. 1(c) and 1(d) in the main text.

Figures S3(a) and (b) show the temperature dependence of the magnetic susceptibilities of the perpendicular and parallel components of spins to the external magentic field applied along $z$-axis, respectively. The inset in Fig. S3(b) is the averaged magnetization density. Figures S3(c) and (d) are the temperture dependence of $\bar{Q^2_{\rm in}}$ and $\bar{Q^2_{\rm out}}$, respectively. The expressions of $\bar{Q^2_{\rm in}}$ and $\bar{Q^2_{\rm out}}$ are given in Eq. (7) in the main text. We emphasize here that all of these results are qualitatively similar to the ones in the triangular lattice discussed in the main text, which indicates that these behaviors are inherent to the ferroquadrupolar phase and independent of the lattice geometry.

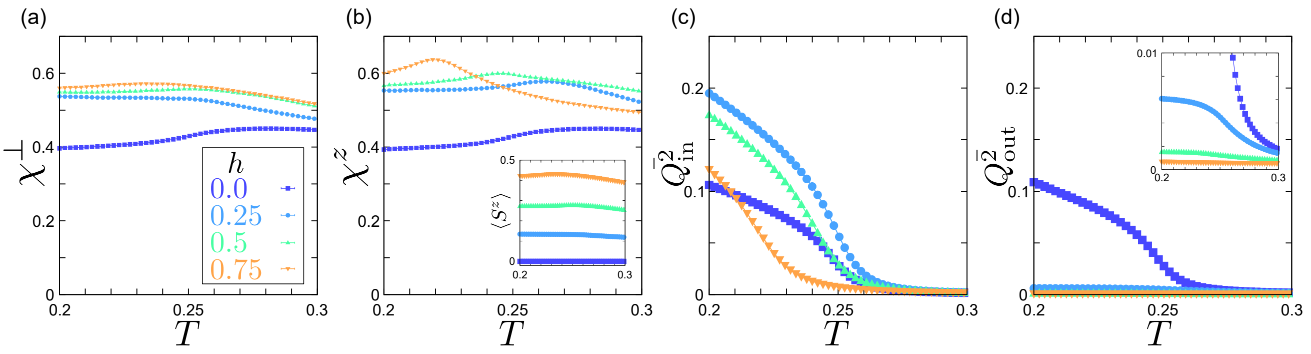


FIG. S3. Detailed results of the sSU(3)-MC simulation for the ferroquadrupolar phase in $L = 32$ square lattice. The parameters are set as $K/J = 2$ and $J, K < 0$, i.e., $(J, K) = (-1/\sqrt{5}, -2/\sqrt{5})$. (a), (b) Temperature dependence of the magnetic susceptibilities (a) perpendicular and (b) parallel to the magnetic field for the various values of $h$. The inset in (b) is the temperature dependence of the averaged magnetization density $\langle S^z \rangle$. (c), (d) Temperature dependence of (c) $\bar{Q}^2_{\rm in}$ and (d) $\bar{Q}^2_{\rm out}$ (Eq. (7) in the main text). The inset in (d) shows the enlarged view in the small $\bar{Q}^2_{\rm out}$ region.
